# Supplementary material for: Non-adiabatic modulation of premixed-flame thermoacoustic frequencies in slender tubes
Source: arXiv:2402.06074 source file (2024-02-08)
Supplement: Supplementary file 1 [file Additional_AuthorInstructions_LaTeX.pdf]

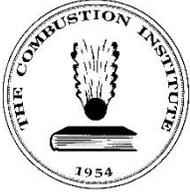

**The Combustion Institute**

5001 Baum Boulevard, Suite 644  
Pittsburgh, Pennsylvania 15213-1851 USA

Ph: (412) 687-1366

Office@CombustionInstitute.org

Fax: (412) 687-0340

CombustionInstitute.org

---

## **Additional Instructions: LaTeX Users, Manuscript Preparation and Word Count**

37th International Symposium on Combustion

Released: 30 September 2017

### **Template Package**

- The template package includes four files:
  - AdditionalInstructionsLaTeX.pdf (this file): Additional instructions to LaTeX Users for manuscript preparation and word count
  - template.tex: LaTeX template for manuscript
  - elsarticle.cls: Elsarticle document class
  - elsarticle-num-PROCI.bst: BibTeX style file for the numbered reference style. This is slightly different from PROCI style, but can also be used

### **Manuscript**

- The submitted manuscript must be single column and double space
- Note that for LaTeX users, separate title page and list of figure captions as described in the file AuthorInstructions\_ManuscriptPrep.pdf are not needed
- Note also that Elsevier does not provide a bibTeX style for the PROCI format. However, the file elsarticle-num-PROCI.bst provided in the package is similar to PROCI style and can also be used.
- In the LaTeX template for manuscript, choose the following option for the manuscript generation
  - `\def\preprint{1}`

### **Word Count**

- Word count is based on two-column paper, which needs to be provided in addition to the main manuscript that is in single column format
- In the LaTeX template for manuscript, choose the following option to generate the two-column paper
  - `\def\wordcount {1}`

- In this two-column format, the first page of the paper only includes the title block and abstract. The maximum paper length including this first page, references, and acknowledgements is 7.5 pages.

### **Submission**

- Both single- and two-column versions of the paper should be uploaded during submission
- Upload the single-column version as “Manuscript”
- Upload the two-column version as “LaTeX 2 Column File”
